# Supplementary material for: Public Perceptions of Fairness Metrics Across Borders
Source: arXiv:2403.16101 source file (2025-05-08)
Supplement: Supplementary file 1 [file 999-supplemenrary.tex]

\section{Additional results}

\subsection{Scores of agreement levels on art project and employee award scenarios}

Figures~\ref{fig:art_boxplot} and~\ref{fig:employee_boxplot} show the distribution of scores for questions assessing participants' agreement or disagreement with the reality of the hiring scenario and the applicability of various fairness metrics in art project and employee award scenarios, respectively. 
Recall that lower scores reflect higher levels of agreement.

Each scenario and fairness metric agreed with the participants.
The difference between fairness metrics is small

\subsection{Full results of correlations between personal attributes and the choice of fairness metrics}

Each participant chose one of the fairness metrics that they considered the most appropriate in each scenario.
We provide the ratio of selected fairness metrics in different personal attributes; country, gender, age, ethnicity, religion, education, and experience. 

\subsubsection{Difference between genders}
\label{sssec:genders}

Figure~\ref{fig:gender}  shows the difference between genders.
The differences are not substantial. 
However, there are certain trends: males had a slightly higher preference for demographic parity compared to females, while females had selected equalized odds more than males.
%The male selects demographic parity more than the female, while the female selects equalized odds more than the male.
People may select advantageous fairness metrics to them. Historically, since males are dominant as candidates in many scenarios (e.g., recruitment), demographic parity may lead to an increase in the number of selected males (i.e., as the number of males increases, the number of selected males increases. See Eq~(\ref{eq:DP}).
Females may consider that people should be selected based on their ability and the number of selected people should depend on the number of qualified candidates in groups.

We also analyze the difference between choices of fairness metrics in genders on each country.
Figures~\ref{fig:hiring_gender_county}--\ref{fig:employee_gender_county} show the results on three scenarios, respectively.
As we mentioned above, males prefer demographic parity more than females, and females prefer equalized odds more than males.
Each country has slightly different trend.
In China, males prefer demographic parity, and females prefer equal opportunity and equalized odds.
In France, females prefer quantitative parity and do not prefer demographic parity. Also, both males and females often choose quantitative parity compared to other countries. 
In Japan, the difference between the ratios of demographic parity in males and females is small compared to other countries.
In Japan and the US, males prefer equal opportunity in most scenarios.

This analysis shows that there is no big gap between genders but they have some characteristics between genders in different countries.

\subsubsection{Difference between ethnicity}
Figure~\ref{fig:ethnicity} shows the difference between ethnicity. We compared each ethnicity in the US and Asia. Recall that we did not collect ethnicity in France due to legal issues.
Due to smalls numbers of Black and H/L in Asia and NA/AN, we removed them from analysis.
%and Other, we . ethnicity from the analysis if the small numbers of participants such as Black and H/L in Asia.

From these results, we can see that even if ethnicity is the same, their choices are different between countries.
In the US, there are no large differences between White, H/L, and Black, while Asian has different trends in the hiring scenario.
On the other hand, in the art project and employee award scenarios, H/L has different trends compared to others. 
In Japan and China, White often selects quantitative parity and Asian often selects demographic parity and equal opportunity.
Therefore, we can consider that the current (and historical) situations of each ethnicity are different in each country.

\subsubsection{Difference between religions}
Figure~\ref{fig:religion} shows the difference between religions. We compared people affiliated with the major and no religions in each country.
The results reveal only minor discrepancies between major and no religions in all countries. 
This observation may imply that cultural influences from major religions might impact even those who do not actively practice the religion. 
For instance, in Japan, despite a high proportion of no religions, Buddhist practices significantly influence cultures, such as seasonal events and funerals.

Furthermore, when comparing the preferences of participants from different countries who share the same major religions, we observed notable dissimilarities. These differences also show the stronger influence of national context than religious affiliation. This shows the impact of country-specific factors is larger than religious influences in the choice of fairness metrics.

% There are a small difference between the major and non-religions in all country.
% This can be considered that even if they have no religions, they may be affected from the major religions in their countries. For example, in Japan, although no religions are dominant, most funerals are held in Buddhism style.
% When we compare the difference between countries with the same major religions, they are not similar if their countries are different. 
% From this result, we can confirm that countries have a larger impact than religions.

\subsubsection{Difference between ages}
Figure~\ref{fig:age} shows the difference between ages. 
It has similar trends that equal opportunity is frequently selected for all ages in most scenarios.
There are two characteristics; 20s often select quantitative parity than others, and 30s and 40s select demographic parity.

First, in terms of the 20s, it might increase the awareness for affirmative action to the hiring balance between genders.
Second, in terms of 30s and 40s, they are often large numbers among ages (see Table~\ref{tab:demographics_age_gender_eth_rel}), so they may select the advantageous fairness metrics for them.

\subsubsection{Difference between educations}
Figure~\ref{fig:education} shows the difference between education. 
Notably, ``less than HS'' and ``some post-secondary'' often select quantitative parity, in particular, hiring and employee award scenarios.
A bachelor's degree often requires many cases such as hiring.
It may affect the choice of fairness metrics in ``less than HS'' and ``some post-secondary''.

\subsubsection{Difference between experiences}
Figure~\ref{fig:experience} shows the difference between experiences. 
There are no clear trends among experiences.
Candidates with non-applicable slightly prefer quantitative parity and others.
Since most candidates belong to non-applicable, it may be better to divide this group into fine groups in order to understand their trends.

 \begin{figure*}[!t]
 \centering
    \begin{minipage}[t]{0.24\linewidth}
        \centering
        \includegraphics[width=1.0\linewidth]{image/allcandidate/art_china_boxplot.pdf}
       \subcaption{China}
       \label{fig:art_boxplot_china}
    \end{minipage}
    \begin{minipage}[t]{0.24\linewidth}
        \centering
        \includegraphics[width=1.0\linewidth]{image/allcandidate/art_france_boxplot.pdf}
        \subcaption{France}
        \label{fig:art_boxplot_japan}
    \end{minipage}
    \begin{minipage}[t]{0.24\linewidth}
        \centering
        \includegraphics[width=1.0\linewidth]{image/allcandidate/art_japan_boxplot.pdf}
        \subcaption{Japan}
        \label{fig:art_boxplot_france}
    \end{minipage}
    \begin{minipage}[t]{0.24\linewidth}
    \centering
    \includegraphics[width=1.0\linewidth]{image/allcandidate/art_usa_boxplot.pdf}
    \subcaption{US}
    \label{fig:art_boxplot_us}
    \end{minipage}
%   \vspace{-1.6 mm}
\caption{Scores of answers for art project scenario}
%\vspace{-3 mm}
\label{fig:art_boxplot}
\end{figure*}

 \begin{figure*}[!t]
 \centering
    \begin{minipage}[t]{0.24\linewidth}
        \centering
        \includegraphics[width=1.0\linewidth]{image/allcandidate/employee_china_boxplot.pdf}
       \subcaption{China}
       \label{fig:employee_boxplot_china}
    \end{minipage}
    \begin{minipage}[t]{0.24\linewidth}
        \centering
        \includegraphics[width=1.0\linewidth]{image/allcandidate/employee_france_boxplot.pdf}
        \subcaption{France}
        \label{fig:employee_boxplot_japan}
    \end{minipage}
    \begin{minipage}[t]{0.24\linewidth}
        \centering
        \includegraphics[width=1.0\linewidth]{image/allcandidate/employee_japan_boxplot.pdf}
        \subcaption{Japan}
        \label{fig:employee_boxplot_france}
    \end{minipage}
    \begin{minipage}[t]{0.24\linewidth}
    \centering
    \includegraphics[width=1.0\linewidth]{image/allcandidate/employee_usa_boxplot.pdf}
    \subcaption{US}
    \label{fig:employee_boxplot_us}
    \end{minipage}
%   \vspace{-1.6 mm}
\caption{Scores of answers for employee award scenario}
%\vspace{-3 mm}
\label{fig:employee_boxplot}
\end{figure*}

\input{image/result_gender}
\input{image/result_ethnicity}
\input{image/result_religions}
\input{image/result_age}
\input{image/result_education}
\input{image/result_experience}
